# Supplementary material for: Chirality in the Kagome Metal CsV$_3$Sb$_5$
Source: arXiv:2408.03750 source file (2024-08-07)
Supplement: Supplementary file 1 [file KagomeCsV3Sb5_supplement_v2.tex]

\documentclass[aps,prl,twocolumn,superscriptaddress,10pt]{revtex4-1}
\usepackage{graphicx}				% need for figures
\usepackage{epsfig}
\usepackage{amsmath,amsthm} % need for subequations
\usepackage{color}
\usepackage{verbatim}				% useful for program listings
\usepackage{ulem}
\raggedbottom          		  % don't add extra vertical space

\bibliographystyle{apsrev4-1}

\begin{document}

\bibliographystyle{prlsty}

\title{Supplemental Material: \\
Chirality in the Kagome Metal CsV$_3$Sb$_5$}

\author{H.J. Elmers}\email{elmers@uni-mainz.de}
\affiliation{Institut f\"{u}r Physik, Johannes Gutenberg-Universit\"{a}t, Staudingerweg 7, D-55128 Mainz, Germany}

\author{O. Tkach}
\affiliation{Institut f\"{u}r Physik, Johannes Gutenberg-Universit\"{a}t, Staudingerweg 7, D-55128 Mainz, Germany}
\affiliation{Sumy State University, Kharkivska 116, 40007 Sumy, Ukraine}

\author{Y. Lytvynenko}
\affiliation{Institut f\"{u}r Physik, Johannes Gutenberg-Universit\"{a}t, Staudingerweg 7, D-55128 Mainz, Germany}
\affiliation{Institute of Magnetism of the NAS and MES of Ukraine, 03142 Kyiv, Ukraine}

\author{P. Yogi}
\affiliation{Institut f\"{u}r Physik, Johannes Gutenberg-Universit\"{a}t, Staudingerweg 7, D-55128 Mainz, Germany}

\author{M. Schmitt}
\affiliation{Diamond Light Source Ltd., Didcot OX11 0DE, United Kingdom}
\affiliation{Physikalisches Institut and Würzburg-Dresden Cluster of Excellence ct.qmat, Julius-Maximilians-Universität, D-97074 Würzburg, Germany}

\author{D. Biswas}
\affiliation{Diamond Light Source Ltd., Didcot OX11 0DE, United Kingdom}

\author{J. Liu}
\affiliation{Diamond Light Source Ltd., Didcot OX11 0DE, United Kingdom}

\author{S. V. Chernov}
\affiliation{Deutsches Elektronen-Synchrotron DESY, 22607 Hamburg, Germany}

\author{M. Hoesch}
\affiliation{Deutsches Elektronen-Synchrotron DESY, 22607 Hamburg, Germany}

\author{D. Kutnyakhov}
\affiliation{Deutsches Elektronen-Synchrotron DESY, 22607 Hamburg, Germany}

\author{N. Wind}
\affiliation{Deutsches Elektronen-Synchrotron DESY, 22607 Hamburg, Germany}
\affiliation{Institut für Experimentelle und Angewandte Physik, Christian-Albrechts-Universität zu Kiel, 24098 Kiel, Germany}

\author{L. Wenthaus}
\affiliation{Deutsches Elektronen-Synchrotron DESY, 22607 Hamburg, Germany}

\author{M. Scholz}
\affiliation{Deutsches Elektronen-Synchrotron DESY, 22607 Hamburg, Germany}

\author{K. Rossnagel}
%\affiliation{Deutsches Elektronen-Synchrotron DESY, 22607 Hamburg, Germany}
\affiliation{Institut für Experimentelle und Angewandte Physik, Christian-Albrechts-Universität zu Kiel, 24098 Kiel, Germany}
\affiliation{Ruprecht Haensel Laboratory, Deutsches Elektronen-Synchrotron DESY, 22607 Hamburg, Germany}

\author{A. Gloskovskii}
\affiliation{Deutsches Elektronen-Synchrotron DESY, 22607 Hamburg, Germany}
\author{C. Schlueter}
\affiliation{Deutsches Elektronen-Synchrotron DESY, 22607 Hamburg, Germany}

\author{A. Winkelmann}
\affiliation{Academic Centre for Materials and Nanotechnology, 
AGH University of Krakow, 30059 Kraków, Poland
}

\author{A.-A. Haghighirad}
\affiliation{
Institute for Quantum Materials and Technologies, Karlsruhe Institute of Technology, 76021
Karlsruhe, Germany}

%\author{more authors?}
%\affiliation{more Instituts?}

\author{T.-L. Lee}
\affiliation{Diamond Light Source Ltd., Didcot OX11 0DE, United Kingdom}

\author{M. Sing}
\affiliation{Physikalisches Institut and Würzburg-Dresden Cluster of Excellence ct.qmat, Julius-Maximilians-Universität, D-97074 Würzburg, Germany}

\author{R. Claessen}
\affiliation{Physikalisches Institut and Würzburg-Dresden Cluster of Excellence ct.qmat, Julius-Maximilians-Universität, D-97074 Würzburg, Germany}

\author{M. Le Tacon}
\affiliation{
Institute for Quantum Materials and Technologies, Karlsruhe Institute of Technology, 76021
Karlsruhe, Germany}

\author{J. Demsar}
\affiliation{Institut f\"{u}r Physik, Johannes Gutenberg-Universit\"{a}t, Staudingerweg 7, D-55128 Mainz, Germany}

\author{G. Sch{\"o}nhense}
\affiliation{Institut f\"{u}r Physik, Johannes Gutenberg-Universit\"{a}t, Staudingerweg 7, D-55128 Mainz, Germany}

\author{O. Fedchenko}
\affiliation{Institut f\"{u}r Physik, Johannes Gutenberg-Universit\"{a}t, Staudingerweg 7, D-55128 Mainz, Germany}

\keywords{}
%\pacs{79.60-i, 73.20-r, 75.25-j, 75.70-i}

\date{\today}

%\begin{abstract}

%Using circularly polarized X-rays, we found a non-trivial circular dichroism in the angular distribution of the valence band photoemission for CsV$_3$Sb$_5$, breaking the time-reversal symmetry of the electronic states. 
%The circular dichroism vanishes for temperatures above the charge density wave transition in this compound, suggesting a relationship between the broken symmetry and the charge order.
%In the X-ray photoelectron diffraction patterns, this is accompanied by a broken mirror symmetry.
%The experimental results indicate an orbital loop current order arising from van Hove singularities related to orbital magnetic moments.

%\end{abstract}

\maketitle

\section{Experimental}

The hexagonal CsV$_3$Sb$_5$ structure and the experimental geometries for the photoemission experiments are shown in Figs.~\ref{Fig1}(a) and \ref{Fig1}(b), respectively. CsV$_3$Sb$_5$ consists of a planar arrangement of V atoms forming a kagome lattice consisting of three sets of parallel lines of V atoms (red) with Sb atoms (gray) as nearest neighbors. The V-Sb planes are separated by Cs atoms, thus forming an electronically two-dimensional lattice.  

The single crystals were freshly cleaved in ultrahigh vacuum.
Circular dichroism experiments in the soft x-ray range were performed 
at the soft x-ray ARPES endstation of Beamline I09 at Diamond Light Source, 
UK~\cite{Schmitt2024}.
%at the endstation of the soft x-ray branch of beamline I09 at the Diamond Light Source,  
%The electron analyzer was a large single hemispherical spectrometer. 
The angle of incidence for the circularly polarized x-rays was $\theta = 22.5^{\circ}$ with respect to the sample surface, 
which was oriented to align the $\Gamma$-M-L plane with the incident beam [see Fig.~\ref{Fig1}(b)]. 
In this case, the total energy resolution was set to 50~meV. 

In addition, soft x-ray photoemission experiments with the time-of-flight momentum microscope at the soft x-ray beamline P04 at PETRA III, DESY, Germany~\cite{Tkach2024}, were performed with the total energy resolution set to 34~meV. We used 330~eV x-rays (corresponding to $k_z=13.7G_{001}$) and the same angle of incidence $\theta = 22.5^{\circ}$. In this case, however, the plane of incidence was along the $\Gamma$-K-H plane [see Fig.~\ref{Fig1}(b)]. 

We used throughout this article the Brillouin zone definition of the high 
temperature phase $T>T_{\rm CDW}$ as shown in Fig.~\ref{Fig1}(c).

\begin{figure}
\includegraphics[width=\columnwidth]{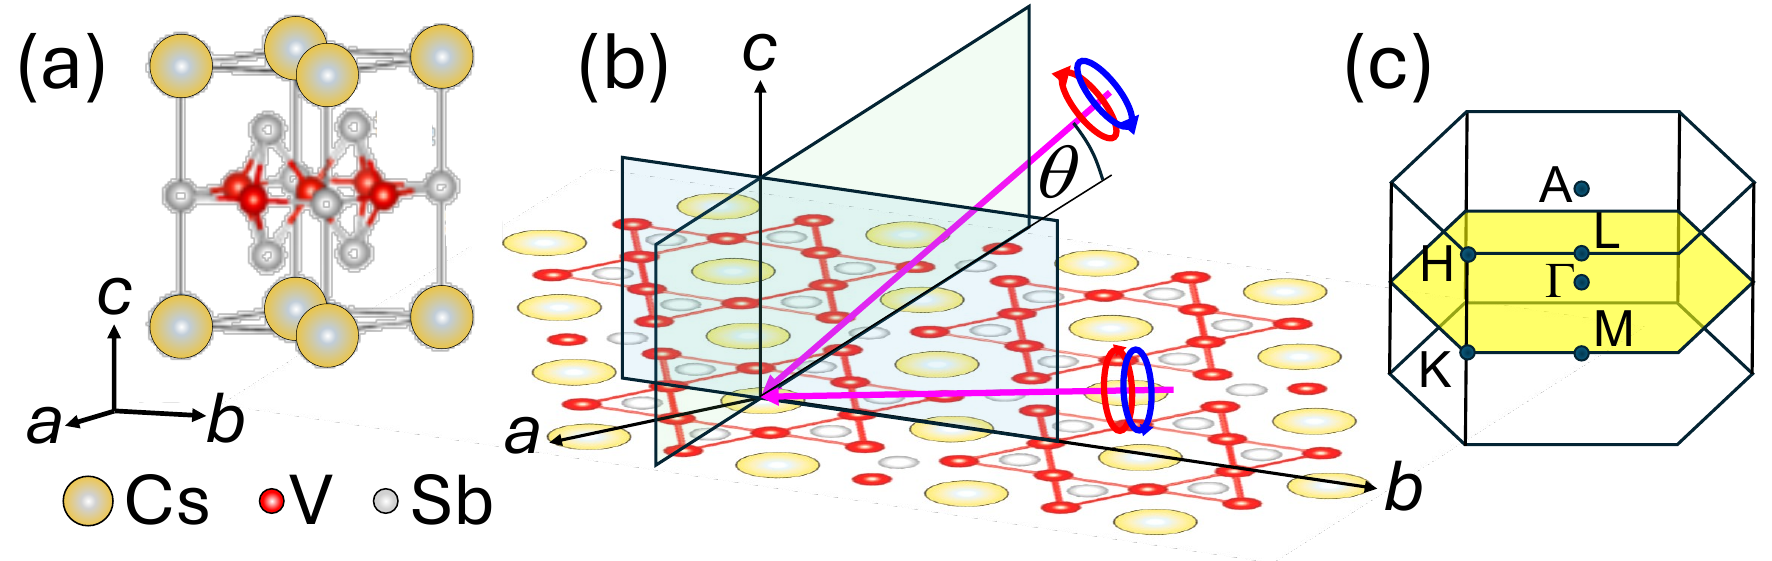}
\caption{\label{Fig1} 
(a) Hexagonal unit cell of CsV$_3$Sb$_5$ in the normal state with unit vectors $a$, $b$, and $c$. The angle between $a$ and $b$ is 60$^{\circ}$.
(b) Experimental geometry. The circularly polarized x-rays impigne on the (001) surface at an angle $\theta$ within the $b-c$ plane or 90$^{\circ}$ rotated.
(c) Brillouin zone of CsV$_3$Sb$_5$ in the high temperature phase with marked high-symmetry points. The high-temperature phase notation was used throughout the paper.
%(sample azimuth rotated by 90 degrees).
%(c) Single plane of the V atoms constituting the Kagome lattice. Small arrows indicate the loop current order. The resulting orbital moments (blue arrows) form a 2x2 superstructure. The corresponding Wigner-Seitz cell is indicated in green as compared to the normal state cell indicated in red. Red and green arrows indicate the corresponding unit vectors along the $a$-axis.
%(d) Reciprocal space representation of the Fermi surface.
%(grey level is proportional to the photoemission intensity). 
%Green and red hexagons indicate the Brillouin zones of the %normal state structure (red) and the 2x2 superstructure (green).
%Green and red arrows mark the corresponding reciprocal lattice vectors. The blue arrows indicate the expected orbital moments near the M-points where the Fermi wave vector and the $\Gamma$ points of the 2x2 superstructure coincide.
}
\end{figure}

\section{X-ray photoelectron diffraction (XPD)}

\begin{figure*}
\includegraphics[width=\textwidth]{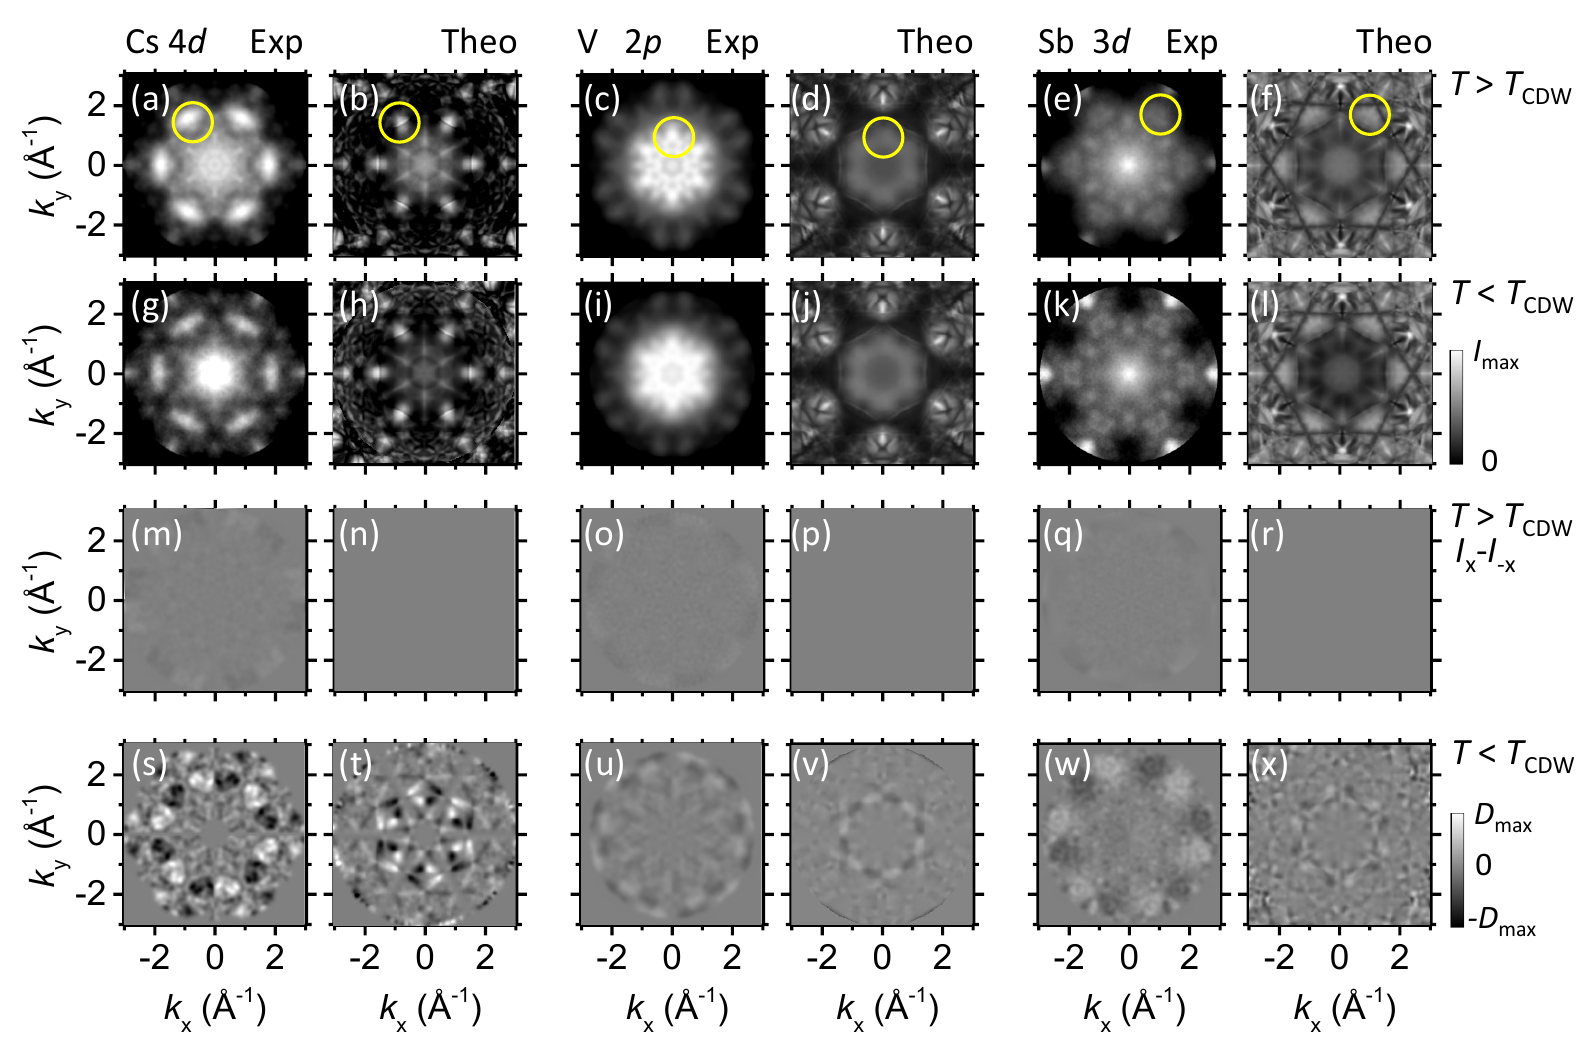}
\caption{\label{Fig5} 
X-ray photoelectron diffraction of CsV$_3$Sb$_5$ measured at a photon energy of 6~keV and for $T>T_{\rm CDW}$ (first row) and $T<T_{\rm CDW}$ (second row), respectively. 
Comparison of  experimental (a,c,e,g,i,k) and theoretical  (b,d,f,h,j,l) data. Yellow circles highlight identical positions of theoretical and experimental data. 
(m,o,q,s,u,w) Difference of original data from (a,c,e,g,i,k) and data mirrored at $k_x=0$ to emphasize the broken mirror symmetry. (n,p,r,t,v,x) Similar data for the calculated results.
The photoemission intensity is normalized to the maximum intensity $I_{\rm max}$ in each image. For the color scale $D_{\rm max}$ is set to 0.04.
}
\end{figure*}

\begin{figure*}
\includegraphics[width=0.7\textwidth]{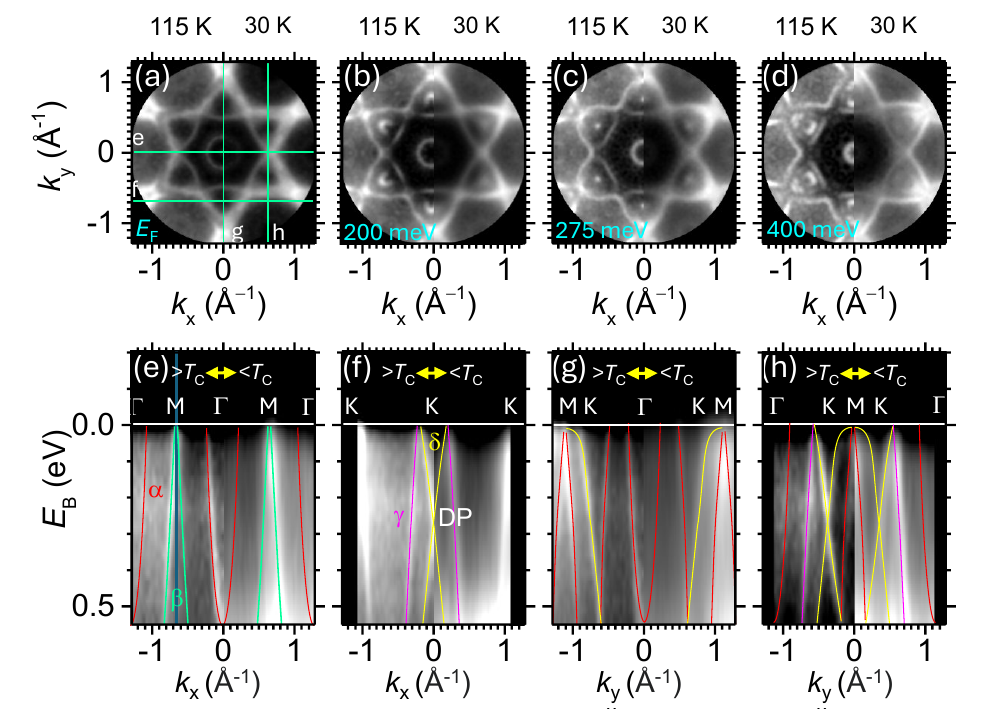}
\caption{\label{Fig3} 
(a-d) Temperature dependence of band dispersion. Constant energy sections of the photoemission intensities in the $k_x - k_y$ plane at the indicated binding energies, measured at a photon energy of 250 (210)~eV. 
(e-h) Band dispersions along the indicated high symmetry directions in reciprocal space.
Data on the left of each panel are measured for $T>T_{CDW}$ (250~eV) and on the right for $T<T_{CDW}$ (210~eV). 
}
\end{figure*}

\begin{figure*}
\includegraphics[width=\textwidth]{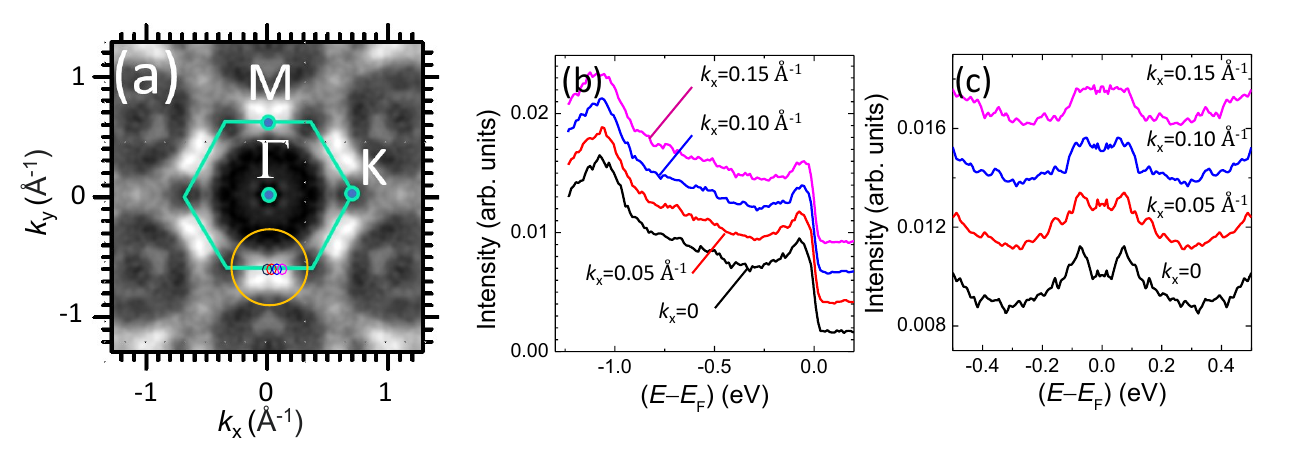}
\caption{\label{Fig_supp_2} 
(a) Fermi surface of CsV$_3$Sb$_5$ from Fig.~4(a) of the main text. Colored circles in the center of the larger yellow circle near the M-point mark positions for the EDCs.
(b) EDCs for distinct $k_{x}$ values indicated in (a) along the M-K direction with $k_x=0$ denoting the M-point.
(c) Sum of the EDCs from (b) and the same EDCs mirrored at the Fermi energy.
The minimum at the Fermi level indicates the energy gap at the M-point.
}
\end{figure*}

Figure~\ref{Fig5} shows experimental and calculated XPD patterns for all three core levels.
All core levels show a pronounced XPD pattern with a sixfold symmetry.
The Cs $4d$ pattern [Fig.~\ref{Fig5}(a)] shows an inner sixfold star in a vertical orientation and an outer ring of high intensity peaks in a straddled orientation (circle). This is in agreement with the pattern calculated using a Bloch wave approach on an XRD-determined crystal structure in the normal state of CsV$_3$Sb$_5$ [Fig.~\ref{Fig5}(b)].
Below the CDW transition,  the inner star has a lower intensity [Fig.~\ref{Fig5}(g)], in agreement with the Bloch wave calculation for the $(2\times 2\times 4)$  
%a 3-dimensional
CDW reconstruction  [Fig.~\ref{Fig5}(h)] (Structural data from Ref.~\cite{Kautzsch2023,Ortiz2021a}).
To highlight the broken mirror symmetry (chirality) of the XPD pattern, we plot the difference $I(k_x,k_y)-I(-k_x,k_y)$ in Fig.~\ref{Fig5}(m,s). 
For 115~K the difference is zero within error limits, indicating mirror symmetry. For 30~K,
the difference also shows a six-fold symmetry. 
However, the mirror symmetry of the pattern is broken.
A detailed inspection of the measured XPD pattern in Fig.~\ref{Fig5}(g) at 30~K shows that
this symmetry breaking originates from a counterclockwise bending of the tips of the inner star and a corresponding lower intensity on the clockwise side of the tip. 
A similar symmetry breaking also shows up in the calculated pattern
shown in Fig.~\ref{Fig5}(t). The mirror symmetric structure for $T>T_{\rm CDW}$ results in a mirror symmetric diffraction pattern as shown in Fig.~\ref{Fig5}(n).

A similar analysis was performed for the V $2p$ and Sb $3d$ XPD patterns.
In the case of V $2p$ [Fig.~\ref{Fig5}(c,i,d,j)] and Sb $3d$ [Fig.~\ref{Fig5}(e,f,k,l)] 
the difference between $T_L=30$~K and $T_H=115$~K is very small for both experimental and theoretical data.
For the Sb $3d$ XPD patterns, we observe a similarly reduced central intensity for $T_L$ as compared to $T_H$ as in the case of Cs $4d$.
%In the case of Sb $3d$ no breaking of the mirror symmetry is visible.
The difference images reveal that all low temperature patterns are chiral 
[Fig.~\ref{Fig5}(s,u,w)] in agreement with calculations [Fig.~\ref{Fig5}(t,v,x)] 
With values up to 0.04. The differences are significantly smaller for V $2p$ and Sb $3d$, see grey level bar. Since the structural changes only affect the V and partly the Sb atomic positions, the scattering rather than the emitter atoms determine the diffraction patterns.
A difference in the actual and assumed atomic positions could explain the remaining differences between experiment and theory.

\section{Details of the electronic band dispersions}

Figure~\ref{Fig3} shows the Fermi surface and the band dispersion with an energy resolution of 50~meV, measured at 30~K and 115~K.
The high (low) temperature data were measured at a photon energy of 
250~eV (210~eV), where both photon energies correspond to an integer perpendicular reciprocal lattice vector.

In agreement with the theory and previous ARPES measurements
we can identify the main band features.
The sections across the $\Gamma$-K-M directions [Fig.~\ref{Fig3}(g,h)]
show the van Hove singularities (vHSs) at the M-point near the Fermi energy, which have a saddle point nature. 
vHS-1 is indicated by the flat yellow $\delta$-band at the M-point in 
Fig.~\ref{Fig3}(g,h). Along the perpendicular direction across the M-point Fig.~\ref{Fig3}(e), it is connected to an electron-like parabola, which is unoccupied at the M-point %(better visible in Fig.~\ref{Fig4}(d))
but acquires a higher binding energy towards the K-point.
At the K-point the band marked by the yellow line forms a Dirac cone with a Dirac point (DP) at a binding energy of 275~meV. This is shown in Figs.~\ref{Fig3}(c,f,h). 
vHS-2 is formed by the $\alpha$-band at the M-point (marked by the red line) with larger dispersion. In the perpendicular $\Gamma$-M direction [Fig.~\ref{Fig3}(e)] it forms an electron-like parabola with a maximum binding energy of less than 100~meV. 
%This can be also clearly observed in Fig.~\ref{Fig4}(d).
vHS-3 at the M-point is connected to the lower Dirac cone at the K-point.
It is outside the measured energy range.
vHS-4 is related to the $\beta$-band (marked by the green line) [Fig.~\ref{Fig3}(e)] with the vHS located above the Fermi level. In the orthogonal direction 
but away from the M-point, this band deforms into the $\gamma$-band (marked by the purple line) shown in Fig.~\ref{Fig3}(f).
Thus, vHS-1 and vHS-2 exhibit an electron-like state along the M-K direction and a hole-like state along the orthogonal M-$\Gamma$ direction and vice versa in the case of vHS-3 and vHS-4~\cite{Wu2024,Hu2022b,Kang2022}. 

The flat dispersion of vHS-1 (yellow-marked $\delta$-band in Fig.~\ref{Fig3}(h)) extends over more than half of the K-M path and indicates
a higher-order nature of this van Hove singularity~\cite{Wu2024,Hu2022b,Kang2022}. 
%40,41 from Ref. https://doi.org/10.1038/s41535-023-00599-y

From the polarization-dependent ARPES measurements reported in
Ref.~\cite{Hu2023} the orbital character of the states forming the van Hove singularities could be identified.
The flat band of vHS-1 (yellow-marked $\delta$-band) 
was assigned to V $d_{x^2-y^2}/d_{z^2}$ orbitals.
vHS-2 is formed by $d_{yz}$-orbitals and vHS-2 by $d_{xy}$-orbitals. 
These van Hove singularities are related to 
the mirror-invariant V sublattice~\cite{Hu2022b}. 
The Bloch states associated with vHS-1, vHS-2 and vHS-3
at the M point are characterized by $A_g$, $B_{2g}$ and $B_{1g}$ irreducible representations with 
inversion-even parity. 
In contrast, vHS-4 corresponds to the $B_{1u}$ irreducible
representation, which is inversion-odd.
vHS-4 arises from two sublattices, corresponding to a
sublattice-mixed type of van Hove singularity~\cite{Hu2022b,Kang2022,Wu2021},
which  is
characterized by eigenstates that are evenly distributed over two
of the three sublattices for each M-point.

At temperatures below $T_{CDW}$ the CDW in CsV$_3$Sb$_5$ 
leads to a reconstruction of the electronic structure
as has been observed by ARPES~\cite{Hu2022c,Kang2022,Luo2022,Lou2022}.
%42–44,48–50.
The in-plane $2\times2$ modulation 
 results in the folding of the
pristine Brillouin zone [see Fig.~1(c) of the main text]. 
The CDW-induced band
folding has been observed as an electron-like band around the $\Gamma$-point that has been back-folded from the M-point~\cite{Jiang2023,Luo2022a}. 
In our case, the intensity near the $\Gamma$-point of the $\alpha$-band is already very low at 210~eV and there is no intensity inside the ring around
$\Gamma$.
In contrast, we observe the band gap associated with the in-plane CDW modulation along the $\Gamma$-K direction [Fig.~\ref{Fig3}(f,h)], which is consistent with previous experimental~\cite{Hu2022c}
%42,48,
and theoretical~\cite{Mielke2022} results.

The band reconstructions in the
ring near the $\Gamma$-point, caused by a hybridization of
the Sb $p$-orbitals and the V $d$-orbitals, are not visible. 
On the other hand, the
triangular constant-energy contours around the K-point 
seem to expand in the CDW phase [Fig.~\ref{Fig3}(b)] as observed previously. 
Presumably, the shift of the vHS bands contributing to the band reconstructions is too small to be identified with the energy resolution of this experiment. This is also true for the $(2\times 2\times 4)$  CDW reconstruction expected from previous work
%, where the 3-dimensional nature of the CDW in CsV$_3$Sb$_5$ was 
%emphasized
~\cite{Hu2022c,Kang2022}.
%42,43.

It has been pointed out that CDW-induced band reconstructions observed by
ARPES~\cite{Hu2022c,Kang2022} % 42,43 
may be influenced by the sample
preparation and precise composition. However, the coexistence of
the Star-of-David and inverse Star-of-David reconstructions in the CDW state is demonstrated by XRD~\cite{Xiao2023,Ortiz2021},
%45,55,
nuclear quadrupole resonance (NQR)~\cite{Feng2023}, and nuclear magnetic
resonance (NMR)~\cite{Frassineti2023} measurements.

\hspace{20 cm}

\section{Energy gaps}

Energy distribution curves (EDCs) at the M-point and along the M-K direction 
at $k_x=0.05, 0.1$, and $0.15$~\AA$^{-1}$ show a systematic variation of the maximum intensity at or slightly below $E_F$ [Fig.~\ref{Fig_supp_2}(b)].
To emphasize these changes, we plot the EDCs symmetrized at the Fermi level [Fig.~\ref{Fig_supp_2}(c)] as described in Ref.~\cite{Luo2022a}.
In this case, an energy gap appears as an intensity minimum at $E_F$ framed by two intensity maxima.
Indeed, we observe an energy gap of 80~meV in the close vicinity of the M-point, which closes at a larger distance from the M-point (c).
This observation is in good agreement with previously reported results~\cite{Hu2023,Luo2022a}.

%\section{Discussion}

\bibliographystyle{apsrev4-1}
%\bibliography{CsV3Sb5}
%merlin.mbs apsrev4-1.bst 2010-07-25 4.21a (PWD, AO, DPC) hacked
%Control: key (0)
%Control: author (72) initials jnrlst
%Control: editor formatted (1) identically to author
%Control: production of article title (-1) disabled
%Control: page (0) single
%Control: year (1) truncated
%Control: production of eprint (0) enabled
%

\end{document}
